# Supplementary material for: Angular analysis of the $B^+\to\pi^+\mu^+\mu^-$ decay
Source: arXiv:2604.21987 source file (2026-09-25)
Supplement: Supplementary file 1 [file appendix.tex]

% ===============================================================================
% Purpose: appendix to the standard template: standard symbol alises from Ulrik
% Author: Tomasz Skwarnicki
% Created on: 2009-09-24
% ===============================================================================

%{\noindent\normalfont\bfseries\Large Appendices}
\section*{Appendices}

\appendix
